# Supplementary material for: A model predictive control (MPC)-integrated multiphase immersed boundary (IB) framework for simulating wave energy converters (WECs)
Source: arXiv:2206.07732 source file (2022-06-15)
Supplement: Supplementary file 1 [file Appendix.tex]

%%%%%%%%%%%%%%%%%%%%%%%%%%%%%%%%%%%%%
\section{Adaptive case}
